# Supplementary material for: RFEPS: Reconstructing Feature-line Equipped Polygonal Surface
Source: arXiv:2212.03600 source file (2022-12-07)
Supplement: Supplementary file 1 [file Appendix.tex]

% \newpage
\appendix

\begin{figure*}[!htp]
	\centering
\begin{overpic}
[width=\linewidth]{more.png}
\end{overpic}
\caption{More reconstruction results of CAD models.}
\label{FIG:moreResults}
\vspace{-4mm}
\end{figure*}

\section{Validation on Feature-line Point Consolidation}
\label{ap:point_consolidation}

RFEPS includes two key modules, including feature-line point consolidation
and RPD reconstruction. In this section, we randomly select 10 shapes from the ABC dataset and use Greedy~\cite{cohen2004greedy} through point set structuring~\cite{PSS} as the reconstruction solver to conduct ablation studies about the effectiveness of the feature-line point consolidation strategy. 
As shown in Table~\ref{ap:tab_consolidation}, our predicted feature-line points significantly improve the reconstruction quality, especially for Model~2, which shows that the proposed feature-line point consolidation strategy is effective.

\section{Validation on RPD based Reconstruction}
\label{ap:RPD_surface}
In this section, we validate the effectiveness of the RPD-based reconstruction
by comparing it with the famous Greedy~\cite{cohen2004greedy} that is also an interpolation-based approach. 
We take the augmented point set (with feature-line points) as the input
and record the ECD and EF1 scores in Table~\ref{ap:tab_rpd}. 
The statistics show that RPD is able to produce an interpolation-based surface with higher accuracy than Greedy.
At the same time, we must point out that the major difference between Greedy and ours lies in that our proposed RPD reconstruction approach is able to yield a watertight manifold, whereas Greedy cannot.

\begin{table}[!htp]
\centering
\caption{
We take Greedy~\cite{cohen2004greedy} through point set structuring~\cite{PSS} as the reconstruction solver to observe the effect of our consolidated feature-line points. We use ``w'' and ``w/o'' to respectively denote ``with consolidation'' and ``without consolidation''. The ablation study shows that our feature-line point consolidation strategy is effective.}
\resizebox{.87\linewidth}{!}{%
\label{ap:tab_consolidation}
\begin{tabular}{l|cc|cc|cc} 
\toprule
{\begin{tabular}[c]{@{}l@{}}\\\end{tabular}} & \multicolumn{2}{c|}{$\mathrm{NC}\uparrow$} & \multicolumn{2}{c|}{$\mathrm{F1} \uparrow$} & \multicolumn{2}{c}{$\mathrm{EF1} \uparrow$} \\ 
\cmidrule{1-7}
% \cmidrule{1-9}
%  & Origin & Consolidation & Origin & Consolidation & Origin & Consolidation \\ 
\makecell[c]{Feature\\points} & w & w/o &  w & w/o  & w & w/o  \\ 
\midrule
Model 1 & 1.000 & \textbf{1.003} & 1.000 & \textbf{1.012} & 1.000 & \textbf{1.355} \\
Model 2 & 1.000 & \textbf{1.011} & 1.000 & \textbf{9.358} & 1.000 & \textbf{28.796} \\
Model 3 & 1.000 & \textbf{1.088} & 1.000 & \textbf{1.720} & 1.000 & \textbf{2.386} \\
Model 4 & 1.000 & \textbf{1.049} & 1.000 & \textbf{5.585} & 1.000 & \textbf{6.235} \\
Model 5 & 1.000 & \textbf{1.003} & 1.000 & \textbf{1.022} & 1.000 & \textbf{1.163} \\
Model 6 & 1.000 & \textbf{1.014} & 1.000 & \textbf{1.122} & 1.000 & \textbf{1.656} \\
Model 7 & 1.000 & \textbf{1.025} & 1.000 & \textbf{1.895} & 1.000 & \textbf{3.163} \\
Model 8 & 1.000 & \textbf{1.024} & 1.000 & \textbf{1.774} & 1.000 & \textbf{3.107} \\
Model 9 & 1.000 & \textbf{1.153} & 1.000 & \textbf{1.743} & 1.000 & \textbf{3.505} \\
Model 10 & 1.000 & \textbf{1.014} & 1.000 & \textbf{1.266} & 1.000 & \textbf{1.310} \\ 
\hline
Mean & 1.000 & \textbf{1.036} & 1.000 & \textbf{1.617} & 1.000 & \textbf{2.182} \\
\bottomrule
\end{tabular}
}
\end{table}

\begin{figure}[!htp]
	\centering
\begin{overpic}
[width=\linewidth]{david.png}
\end{overpic}
\vspace{-3mm}
\caption{Test RFEPS on the David model.}
\label{FIG:ap_david}
\end{figure}
\begin{table}[!htp]
\centering
\caption{We take the augmented point set (with feature-line points) as the input to compare Greedy and our RPD reconstruction in terms of ECD and EF1. We normalize the score of Greedy to~1 for better presentation. At the same time, we must point out that our proposed RPD reconstruction approach is able to yield a watertight manifold whereas Greedy cannot. }
\label{ap:tab_rpd}
\resizebox{\linewidth}{!}{%
\begin{tabular}{l|cc|cc||cc|cc} 
\toprule
\begin{tabular}[c]{@{}l@{}}\\\\\end{tabular} & \multicolumn{2}{c|}{$\mathrm{ECD} \downarrow$} & \multicolumn{2}{c||}{$\mathrm{EF1} \uparrow$} & \multicolumn{2}{c|}{Manifold} & \multicolumn{2}{c}{Watertight} \\ 
\cmidrule{1-9}
\makecell[c]{Reconstruction\\algorithm} & Greedy & RPD & Greedy & RPD & Greedy & RPD & Greedy & RPD \\ 
\hline
Model 1 & 1.000 & \textbf{0.652} & 1.000 & \textbf{1.114} & $\times$ & \checkmark & $\times$ &  \checkmark \\
Model 2 & \textbf{1.000} & 1.125 & \textbf{1.000} & 0.996 & $\times$ & \checkmark& $\times$ &\checkmark  \\
Model 3 & 1.000 & \textbf{0.765} & 1.000 & \textbf{1.033} & $\times$ & \checkmark & $\times$ & \checkmark \\
Model 4 & 1.000 & \textbf{0.752} & 1.000 & \textbf{1.035} & $\times$ &\checkmark  & $\times$ & \checkmark \\
Model 5 & 1.000 & \textbf{0.891} & 1.000 & \textbf{1.023} & $\times$ &\checkmark  & $\times$ &\checkmark  \\
Model 6 & 1.000 & \textbf{0.738} & 1.000 & \textbf{1.025} & $\times$ &\checkmark  & $\times$ &\checkmark  \\
Model 7 & 1.000 & \textbf{0.804} & 1.000 & \textbf{1.079} & $\times$ &\checkmark  & $\times$ & \checkmark \\
Model 8 & 1.000 & \textbf{0.629} & 1.000 & \textbf{1.061} & $\times$ &\checkmark  & $\times$ & \checkmark \\
Model 9 & 1.000 & \textbf{0.854} & 1.000 & \textbf{1.012} & $\times$ &\checkmark  & $\times$ &\checkmark  \\
Model 10 & 1.000 & \textbf{0.674} & 1.000 & \textbf{1.076} & $\times$ & \checkmark & $\times$ & \checkmark \\ 
\hline
Mean & 1.000 & \textbf{0.931} & 1.000 & \textbf{1.036} & \multicolumn{4}{c}{} \\
\bottomrule
\end{tabular}
}
\end{table}

% \begin{figure*}[htp]
% 	\centering
% \begin{overpic}
% [width=\linewidth]{more.png}
% \end{overpic}
% \caption{More reconstruction results of CAD models.}
% \label{FIG:moreResults}
% \vspace{-4mm}
% \end{figure*}

\section{Reconstruction for Non-CAD models}
\label{ap:non_cad_model}
In this paper, we focus on the surface reconstruction problem by assuming that the input point cloud is sampled from a CAD model.
But we must point out that our RFEPS also applies to a general non-CAD model.
In Figure~\ref{FIG:ap_david}, we sample 1500K points from the David model
and visualize the reconstruction result.
From the close-up window, one can see that RFEPS is able to well preserve the feature lines, enabling the reconstructed surface with high fidelity. 

\begin{figure}[!htp]
	\centering
\begin{overpic}
[width=\linewidth]{noise.png}
\put(17,-2){(a)}
\put(50,-2){(b)}
\put(81,-2){(c)}
\end{overpic}
\caption{In order to deal with severe noise, our RFEPS may need a denoising step.
(a)~Noisy inputs. (b)~Denoised results through jet smoothing~\cite{jet}.
(c)~Reconstruction results by RFEPS.}
\label{FIG:ap_noise}
\vspace{-4mm}
\end{figure}

\begin{figure}[!htp]
	\centering
\begin{overpic}
[width=.8\linewidth]{F1.png}
\end{overpic}
\caption{If there exist two feature lines in a very narrow zone.
REFPS may confuse one feature line with the other. }
\label{FIG:FailureCase1}
\vspace{-4mm}
\end{figure}

\section{Noisy Point Cloud Input}
\label{ap:noise}
When the input point cloud has severe noise,
our RFEPS requires a denoising step. 
Here we use the off-the-shelf denoising method~\cite{jet} to preprocess the noisy data.
Figure~\ref{FIG:ap_noise} shows a group of noisy inputs and each of them has 50K points.
It can be seen that as long as the noise is degraded, RFEPS can still produce a high-quality
surface with clean feature-line frames. 

% To cope with a point cloud input with severe noise, we adopt  Then we apply the proposed RFEPS to achieve surface reconstruction. As shown in Figure~\ref{FIG:ap_noise}, given a noisy point cloud input, our method still produces feature line well-preserved reconstruction even with a naive denoising technique~\cite{jet}. Note that the number of points in the point cloud is $50k$ same as the main paper. 
%\ZY{@Rui, can we show more results? to make this part more convincing. Btw, pls zoom in the point cloud input for demonstration. }

\begin{figure}[!htp]
	\centering
\begin{overpic}
[width=\linewidth]{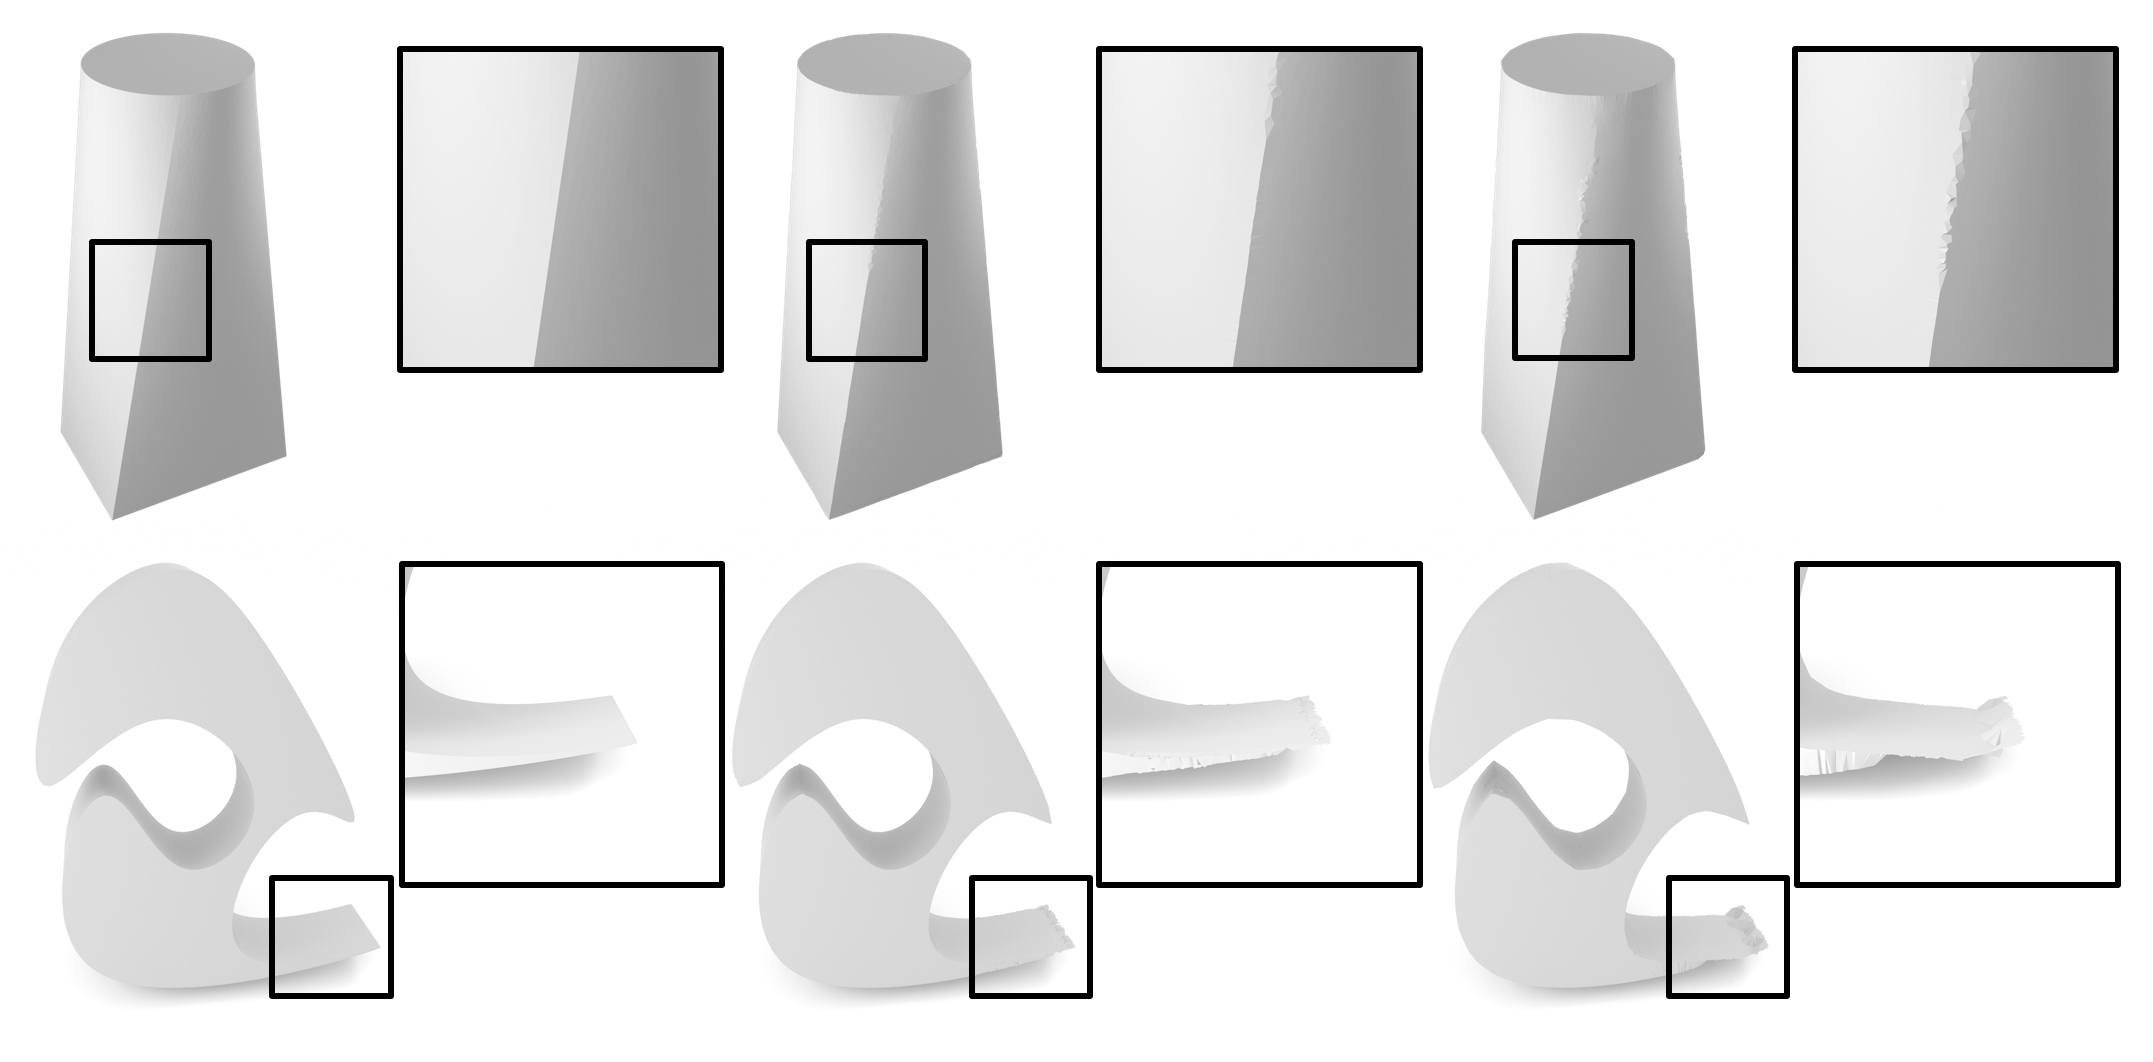}
\put(18,0){\textbf{SPR}}
\put(64,0){\textbf{Ours}}
\end{overpic}
\caption{RFEPS may fail on a model with extremely small dihedral angles.}
\label{FIG:FailureCase2}
\vspace{-2mm}
\end{figure}

\section{More Results}
We provide more reconstruction results of CAD models, see Figure~\ref{FIG:moreResults}.

\section{Failure Cases}
\label{ap:failure_cases}
In this section, we demonstrate two failure cases of REFPS.
First, REFPS, in its current form, supports the dihedral-angle range of $[\pi/6, 5\pi/6]$. 
When the underlying surface has a dihedral angle that is close to $0$ or $\pi$ around the feature line, our method may fail. 
If the dihedral angle is between $[5\pi/6,\pi]$, we omit the existence of feature lines by Eq.~(\ref{equa:FeatureZone}). 
If the dihedral angle is between $[0,\pi/6]$, as Figure~\ref{FIG:FailureCase2} shows,
Poisson reconstruction generates a poor-quality base surface with many unwanted topological holes, which leads to misconnection between points when we run RPD.
Besides, REFPS may fail if thin sheets exist in the given point cloud.
As Figure~\ref{FIG:FailureCase1} shows, there are two feature lines in a very narrow zone.
REFPS cannot distinguish one feature line from the other.
